# Supplementary material for: Traffic4cast at NeurIPS 2021 -- Temporal and Spatial Few-Shot Transfer Learning in Gridded Geo-Spatial Processes
Source: arXiv:2203.17070 source file (2022-04-01)
Supplement: Supplementary file 1 [file main.tex]

\documentclass[pmlr]{jmlr} % W&CP article
 
% The following packages will be automatically loaded:
% amsmath, amssymb, natbib, graphicx, url, algorithm2e

%\usepackage{rotating}% for sideways figures and tables
\usepackage{longtable}% for long tables

% The booktabs package is used by this sample document
% (it provides \toprule, \midrule and \bottomrule).
% Remove the next line if you don't require it.
\usepackage{booktabs}
\usepackage[load-configurations=version-1]{siunitx} % newer version
\usepackage{ulem}
\usepackage{longtable}

\theorembodyfont{\upshape}
\theoremheaderfont{\scshape}
\theorempostheader{:}
\theoremsep{\newline}

\def\t4c{\textit{Traffic4cast}\relax}

\jmlrproceedings{PMLR}{IARAI Report}
\jmlrworkshop{\t4c at NeurIPS 2021 -- Competition Design and Data}

\usepackage{graphicx}
\usepackage{color}
\usepackage{xcolor}
\usepackage{amssymb}
% https://tex.stackexchange.com/questions/3033/forcing-linebreaks-in-url
\PassOptionsToPackage{hyphens}{url}
\usepackage{hyperref}
\usepackage{csquotes}
\usepackage{mdframed}
\usepackage{verbatim}   % for the comment environment
\usepackage{ifthen}
\usepackage{lipsum}
\usepackage{footmisc}
\usepackage{tablefootnote}
\usepackage{microtype}

\let\cite\citep

% if you want to see the todo
\newcommand{\showtodos}{show them}  % comment this line if you don't 
                                    % want to see todo environment
% the todo environment
%
        {%drem
            \ifthenelse{\isundefined{\showtodos}}%
                    {\expandafter\comment}%
                    {\begin{mdframed} \textcolor{red}{{\bf TODO}}}%
                    }%
         {%
            \ifthenelse{\isundefined{\showtodos}}%
                    {\expandafter\endcomment}%
                    {\end{mdframed}}%
          }

\def\t4c{\textit{Traffic4cast}\relax}

\title[\t4c at NeurIPS 2021]{\t4c at NeurIPS 2021 Competition Design and Data -- Supplementary Reference Material\\ {\small \url{http://traffic4cast.ai} -- \url{https://github.com/iarai/NeurIPS2021-traffic4cast}}}

\def\t4c{\textit{Traffic4cast}\relax}

% Alternative format for long lists? https://www.jmlr.org/papers/volume22/20-1307/20-1307.pdf
\author{%
\Name{Moritz Neun}\thanks{Equal contribution}\thanks{Institute of Advanced Research in Artificial Intelligence (IARAI), Vienna, Austria} \Email{moritz.neun@iarai.ac.at}
\AND
\Name{Christian Eichenberger}\footnotemark[1]\footnotemark[2] \Email{christian.eichenberger@iarai.ac.at}
\AND
\Name{Henry Martin}\footnotemark[2]\thanks{Institute of Cartography and Geoinformation, ETH Zurich, Switzerland} \Email{henry.martin@iarai.ac.at}
\AND
\Name{Pedro Herruzo}\footnotemark[2] \Email{pedro.herruzo@iarai.ac.at}
\AND
\Name{Markus Spanring}\footnotemark[2] \Email{markus.spanring@iarai.ac.at}
\AND
\Name{David Jonietz} \thanks{HERE Technologies, Zurich, Switzerland} \Email{david.jonietz@here.com}
\AND
\Name{Fei Tang} \footnotemark[4] \Email{fei.tang@here.com}
\AND
\Name{Aleksandra Gruca}\thanks{Silesian University of Technology, Gliwice, Poland} \Email{aleksandra.gruca@polsl.pl}
\AND
\Name{Michael Kopp}\footnotemark[2] \Email{michael.kopp@iarai.ac.at}
\AND
\Name{David Kreil}\footnotemark[2] \Email{david.kreil@iarai.ac.at}
\AND
\Name{Sepp Hochreiter}\thanks{Machine Learning Institute, Johannes Kepler University Linz, Austria}\footnotemark[2] \Email{sepp.hochreiter@iarai.ac.at}
\AND
}

\date{\today}

\begin{document}
% \tableofcontents
% \clearpage
\setcounter{page}{1}

\maketitle

% \newpage
\begin{abstract}
We here present and discuss the design of the \t4c 2021 competition and its data (\url{www.traffic4cast.ai}).
The manuscript compiles and shares so-far unpublished details from the competition proposal, preparations, and blogs for further reference, which 
are of direct interest to \textit{post hoc} meta or performance analyses, and studies of interpretability such as the {\it Analysis and Interpretability Challenge} of \t4c 2021, \textit{cf.}
\url{https://www.iarai.ac.at/traffic4cast/2021-competition/challenge/#analyticschallenge}. This is demonstrated for a range of analysis perspectives.
\end{abstract}

\section{Introduction}\label{sec:introduction}
More than half of the world's population is living in urban areas. Urbanization is ever growing, with over two thirds of all people expected to live in cities by 2050 \cite{UN_Urbanization_Prospects_2018}. Meanwhile, today's dynamic economies and personal preferences lead to increased demands for mobility, with considerable impact on
the environment, public health, and the running of societies. Hence the question arises how we can best live in urban areas in the future and how we can optimize our use of urban space. A principled discussion will rely on an understanding of the patterns underlying urban traffic flows.
The \t4c competition goes to the heart of this matter, advancing and applying modern machine learning approaches to help understand complex systems like traffic that follow implicit rules, and make successful predictions about future states of such systems. 

After an overview of the competition design for the \t4c 2021 \citep{eichenberger_traffic4cast_2021} we here provide more details and considerations regarding the competition data and metrics. The paper in particular compiles so far unpublished materials from the competition proposal and blogs for further reference, which are of direct interest to \textit{post hoc} meta or performance analyses, as well as studies of interpretability such as the {\it Analysis and Interpretability Challenge} of \t4c 2021, \textit{cf.}
\url{https://www.iarai.ac.at/traffic4cast/2021-competition/challenge/#analyticschallenge}.

\input{supplementary/supplementary}

\section{Conclusion}
In this article, we compiled and shared so-far unpublished details from the competition proposal, preparations, and blogs for further reference, which 
are of direct interest to \textit{post hoc} meta or performance analyses, and studies of interpretability such as the {\it Analysis and Interpretability Challenge} of \t4c 2021, \textit{cf.}
\url{https://www.iarai.ac.at/traffic4cast/2021-competition/challenge/#analyticschallenge}.
This was demonstrated for a range of analysis perspectives: Specifically, we illustrated and discussed possible interpretations of temporal shift in the data, which also motivates the core competition on transfer learning for a temporal domain shift. Complementing temporal shift analysis, we also examined the spatial and temporal heterogeneity of traffic data and assessed data sparsity at different granularity levels, including effects of the city, region, time of day, and collection source (car fleets levels). This highlighted the relevance of the extended competition targeting models robust under a spatio-temporal domain shift.
Last but not least, we demonstrated that a spatial mask of the mean square error to the road network had negligible effects, which implies that models working on the road graph and projecting predictions onto the 3-level spatial gridding (pixel rows, columns, and headings) are not heavily penalized by evaluating by data outside of the road graph.

\end{document}
